# Supplementary material for: Decomposing the dynamics of heterogeneous delayed networks with applications to connected vehicle systems
Source: arXiv:1305.6771 source file (2013-09-27)
Supplement: Supplementary file 1 [file SuppMat_r3.pdf]

# Supplemental material – differentiating the eigenvalues of a parameter dependent matrix


Róbert Szalai

*Department of Engineering Mathematics,*

*University of Bristol, Bristol, BS8 1TR, UK*

Gábor Orosz

*Department of Mechanical Engineering,*

*University of Michigan, Ann Arbor, Michigan 48109 USA*



(Dated: September 27, 2013)

PACS numbers:

The purpose of this Supplemental Material is to show how the eigenvalues of a parameter dependent matrix are differentiated with respect to its parameters. We consider the case when the matrix linearly depends on the parameters and the derivatives are calculated with respect to each parameter when all the parameters are equal.

In the manuscript we introduced the $N$ by $N$ matrix $B_N = \sum_{i,j=1}^{N} \zeta_{ij} A_{ij}$ where $\zeta_{ij} = \mathrm{e}^{-s\,\tau_{ij}}$ with delays $\tau_{ij}$ and each $A_{ij}$ is a matrix that has a single nonzero element $a_{ij}$ in row $i$, column $j$. These matrices build up the $N$-dimensional adjacency matrix $A_N = \sum_{i,j=1}^{N} A_{ij}$. In this form $B_N$ is linearly dependent on the parameters $\zeta_{ij}$. The eigenvalues of $B_N$ are denoted by $\bar{\Lambda}_k$, $k = 1, \ldots, N$ and depend on $\zeta_{ij}$. We are seeking the derivatives of $\bar{\Lambda}_k$ with respect to $\zeta_{ij}$ that appear when considering the Taylor series of the eigenvalues about the point where the delays are identical $\zeta_{ij} = \mathrm{e}^{-s\,T_0} := \zeta_0$. Using Taylor series we extrapolate the case of identical delays to the heterogeneous case.

As a first step we introduce new indices $\ell = 1, \ldots, M = N^2$ to replace $i, j = 1, \ldots, N$. That is, we have the matrixes $A_\ell$ with nonzero elements $a_\ell$, the delays $\tau_\ell$, and the corresponding parameters $\zeta_\ell = \mathrm{e}^{-s\,\tau_\ell}$. Thus, the Taylor series can be written as

$$\bar{\Lambda}_k(\zeta_1, \ldots, \zeta_M) = \sum_{Q=0}^{\infty} \sum_{q_1+\cdots+q_M=Q} \frac{1}{q_1! \cdots q_M!}\, \partial_1^{q_1} \cdots \partial_M^{q_M} \bar{\Lambda}_k\big|_0 \cdot (\zeta_1 - \zeta_0)^{q_1} \cdots (\zeta_M - \zeta_0)^{q_M}\,, \quad (1)$$

where $\partial_\ell^{q_\ell}$ denotes the $q_\ell$-th partial derivative with respect to $\zeta_\ell$ and $\big|_0$ refers to that the derivatives are evaluated at $(\zeta_1, \ldots \zeta_n) = (\zeta_0, \ldots \zeta_0)$. Note that when the delays are the same $\tau_\ell = T_0$, the eigenvalues of $B_N$ are $\bar{\Lambda}_k\big|_0 = \zeta_0 \Phi_k$ where $\Phi_k$ are the eigenvalues of the adjacency matrix $A_N = \sum_{\ell=1}^{M} A_\ell$ that depend solely on $a_\ell$. In the case of identical delays $B_N = \zeta_0 A_N$, so the left and right eigenvectors $w_k\big|_0$ and $v_k\big|_0$, can be chosen independent of $\zeta_0$.

Define $\bar{B}_\ell = B_N - \zeta_\ell A_\ell$, where $\zeta_\ell = \mathrm{e}^{-s\,\tau_\ell}$. Then, the eigenvalue problem can be written as

$$\begin{aligned} \big(\bar{B}_\ell + \zeta_\ell A_\ell - \bar{\Lambda}_k I\big)\, v_k &= 0\,, \\ w_k \big(\bar{B}_\ell + \zeta_\ell A_\ell - \bar{\Lambda}_k I\big) &= 0, \end{aligned} \quad (2)$$

where $\bar{\Lambda}_k, w_k, v_k$ are functions of all $\zeta_\ell$ and $I$ is the $N$-dimensional identity matrix. Differentiating (2) with respect to $\zeta_\ell$ yields

$$\big(A_\ell - \partial_\ell \bar{\Lambda}_k I\big)\, v_k + \big(\bar{B}_\ell + \zeta_\ell A_\ell - \bar{\Lambda}_k I\big)\, \partial_\ell v_k = 0\,. \quad (3)$$

In order to calculate the derivative $\partial_\ell \bar{\Lambda}_k$ we multiply (3) by the left eigenvector $w_k$ from the

left to get

$$\partial_\ell \bar{\Lambda}_k = \frac{w_k A_\ell \, v_k}{w_k v_k}\,. \tag{4}$$

In general, $\partial_\ell \bar{\Lambda}_k$ depends on the delays through the eigenvectors. However, when evaluating this derivative at the point where all the delays are the same, the eigenvectors are delay independent, and consequently $\partial_\ell \bar{\Lambda}_k\big|_0$ only depends on $a_\ell$. The derivative of the eigenvectors can be calculated from (3). Considering the identical delays and substituting the eigenvalues $\bar{\Lambda}_k\big|_0 = \zeta_0 \Phi_k$ we obtain

$$\left(A_\ell - \partial_\ell \bar{\Lambda}_k\big|_0 I\right) v_k\big|_0 + \zeta_0 \left(A_N - \Phi_k I\right) \partial_\ell v_k\big|_0 = 0\,. \tag{5}$$

Hence for identical delays we have the derivatives $\partial_\ell v_k\big|_0 = \frac{1}{\zeta_0}\partial_\ell V_k = \mathrm{e}^{s\,T_0}\partial_\ell V_k$ where $\partial_\ell V_k$ is a solution of (5) for $\partial_\ell v_k\big|_0$ with $\zeta_0 = 1$.

Calculating further derivatives with respect to $\zeta_{\ell_j}$, $j = 1, \ldots, n$ and evaluating the equations at the identical delay case we obtain

$$\begin{aligned}
&- \partial_{\ell_1} \cdots \partial_{\ell_n} \bar{\Lambda}_k\big|_0 v_k\big|_0 - \partial_{\ell_1} \cdots \partial_{\ell_{n-1}} \bar{\Lambda}_k\big|_0 \partial_{\ell_n} v_k\big|_0 - \cdots - \partial_{\ell_1}\partial_{\ell_2} \bar{\Lambda}_k\big|_0 \partial_{\ell_3} \cdots \partial_{\ell n} v_k\big|_0 \\
&+ \sum_{p=1}^{n} \left(A_{\ell_p} - \partial_{\ell_p} \bar{\Lambda}_k\big|_0 I\right) \partial_{\ell_1} \cdots \partial_{\ell_{p-1}} \partial_{\ell_{p+1}} \cdots \partial_{\ell_n} v_k\big|_0 + \zeta_0 \left(A_N - \Phi_k I\right) \partial_{\ell_1} \cdots \partial_{\ell_n} v_k\big|_0 = 0\,.
\end{aligned} \tag{6}$$

Similar to the first derivatives, when multiplying (6) by $w_k$ from the left we can express the derivative as

$$\begin{aligned}
\partial_{\ell_1} \cdots \partial_{\ell_n} \bar{\Lambda}_k\big|_0 = \frac{w_k}{w_k v_k} \Bigg( &\sum_{p=1}^{n} \left(A_{\ell_p} - \partial_{\ell_p} \bar{\Lambda}_k\big|_0 I\right) \partial_{\ell_1} \cdots \partial_{\ell_{p-1}} \partial_{\ell_{p+1}} \cdots \partial_{\ell_n} v_k\big|_0 \\
&- \partial_{\ell_1} \cdots \partial_{\ell_{n-1}} \bar{\Lambda}_k\big|_0 \partial_{\ell_n} v_k\big|_0 - \cdots - \partial_{\ell_1}\partial_{\ell_2} \bar{\Lambda}_k\big|_0 \partial_{\ell_3} \cdots \partial_{\ell n} v_k\big|_0 \Bigg)\,,
\end{aligned} \tag{7}$$

which depends on lower than $n$th order derivatives of the eigenvalue $\bar{\Lambda}_k$ and eigenvector $v_k$. By induction we show that

$$\partial_1^{q_1} \cdots \partial_M^{q_M} \bar{\Lambda}_k\big|_0 = \partial_{\ell_1} \cdots \partial_{\ell_n} \bar{\Lambda}_k\big|_0 = \frac{1}{\zeta_0^{n-1}} \Phi_{k,\ell_1 \cdots \ell_{n-1}} = \mathrm{e}^{s\,(n-1)\,T_0} \Phi_{k,\ell_1 \cdots \ell_{n-1}} \tag{8}$$

and

$$\partial_1^{q_1} \cdots \partial_M^{q_M} v_k\big|_0 = \partial_{\ell_1} \cdots \partial_{\ell_n} v_k\big|_0 = \frac{1}{\zeta_0^{n}} V_{k,\ell_3 \cdots \ell_n} = \mathrm{e}^{s\,n\,T_0} V_{k,\ell_3 \cdots \ell_n} \tag{9}$$

where $q_j = \sum_{p=1,\ell_p=j}^{n} 1$, $Q = \sum_{j=1}^{M} q_j = n$ and $\Phi_{k,\ell_1 \cdots \ell_{n-1}}$, $V_{k,\ell_3 \cdots \ell_n}$ only depend on $a_\ell$. We already know that (8) and (9) hold for $n = 1$. It remains to show that if the assertion holds

for $n-1$ it also holds for $n$. Substituting our assumptions (8) and (9) into (7) we get

$$\partial_{\ell_1}\cdots\partial_{\ell_n}\bar{\Lambda}_k\big|_0 = \frac{w_k}{\zeta_0^{n-1} w_k v_k}\Bigg(\sum_{p=1}^{n}\left(A_{\ell_p} - I\Phi_{k,\ell_p}\right)V_{k,\ell_1\cdots\ell_{p-1}\ell_{p+1}\cdots\ell_n} \\ - \Phi_{k,\ell_1\cdots\ell_{n-1}}V_{k,\ell_n} - \cdots - \Phi_{k,\ell_1\ell_2}V_{k,\ell_3\cdots\ell_n}\Bigg), \tag{10}$$

which proves (8). The same can be shown for the eigenvectors when substituting directly into (6)

$$-\zeta_0^{1-n}\Phi_{k,\ell_1\cdots\ell_n}V_k - \zeta_0^{1-n}\Phi_{k,\ell_1\cdots\ell_{n-1}}V_{k,\ell_n} - \cdots - \zeta_0^{1-n}\Phi_{k,\ell_1\ell_2}V_{k,\ell_3\cdots\ell n} \\ + \zeta_0^{1-n}\sum_{p=1}^{n}\left(A_{\ell_p} - \Phi_{k,\ell_p}I\right)V_{k,\ell_1\cdots\ell_{p-1}\ell_{p+1}\cdots\ell_n} + \zeta_0\left(A_N - \Phi_k I\right)\partial_{\ell_1}\cdots\partial_{\ell_n}v_k\big|_0 = 0. \tag{11}$$

Dividing by $\zeta_0$ proves (9).
